# Supplementary material for: Fast Uplink Grant-Free NOMA with Sinusoidal Spreading Sequences
Source: arXiv:2010.00199 source file (2020-10-01)
Supplement: Supplementary file 1 [file appendix.tex]

\subsection{Proof of Lemma 1}
\label{lemma1}
The received signal at $m^{th}$ subcarrier where $m\in\{1,2, \ \cdots \ M\}$ at $j^{th}$ frame can be expressed as following
\begin{equation}
    y_{m,j} = \sum_{n \in \mathcal{N}} h_n\beta_{n,j}\exp(\irm\omega_n m) + w_{m,j}
    \label{append}
\end{equation}

Hence, if we consider the received signals in each subcarrier $\{m\}_{m=1}^M$ are statistically independent, it will be sufficient to prove that $\mathcal{Z} = \beta_{n,j}h_n \sim \mathcal{CN}(0,\sigma^2)$ is a zero mean complex Gaussian random variable. Now, let us consider the data symbol $\beta_{n,j}$ as a discrete uniform random variable taking values on finite alphabet QPSK constellation $\mathcal{A} = [\ 1 \ \ 1j \ -1 \ -1j \ ]$ whereas $h_n \sim \mathcal{CN}(0,\tau_n)$ is a continuous Gaussian random variable. This is noteworthy that following is valid for any symmetric constellation but for the sake of brevity, QPSK constellation is used without any loss of generality.  

We can write for any $\mathcal{Z}=z$ 
\begin{equation}
   \begin{split}
    \mathrm{Pr}(\beta_{n,j}h_n<z) &= \mathrm{Pr}(\beta_{n,j}h_n<z)\mathrm{Pr}(\beta_{n,j} = 1)+ \nonumber\\ & \mathrm{Pr}(\beta_{n,j}h_n<z)\mathrm{Pr}(\beta_{n,j} = 1\irm) + \nonumber\\ & \mathrm{Pr}(\beta_{n,j}h_n<z)\mathrm{Pr}(\beta_{n,j} = -1) + \nonumber\\ & \mathrm{Pr}(\beta_{n,j}h_n<z)\mathrm{Pr}(\beta_{n,j} = -1\irm)
\end{split} 
\end{equation}
Since all of the symbols in $\mathcal{A}$ are equally probable, we can write
\begin{equation}
    \begin{split}
        \mathrm{Pr}(\beta_{n,j}h_n<z) &= \frac{1}{4}\mathrm{Pr}(h_n<z) + \frac{1}{4}\mathrm{Pr}(h_n>-z) + \nonumber\\ & \frac{1}{4}\mathrm{Pr}(\irm h_n<z) + \frac{1}{4}\mathrm{Pr}(\irm h_n>-z)
    \end{split}
\end{equation}
Due to the symmetry of Gaussian, first two term in above equation yields $\frac{1}{2}\mathrm{Pr}(h_n<z)$. Moreover, since $h_n$ is a zero mean Gaussian, it has zero mean real and imaginary part. With this, along with the symmetry of Gaussian distribution and symmetry of the constellation, the last two terms in above equation yields $\frac{1}{2}\mathrm{Pr}(h_n<z)$. Combining all of this, we get
\begin{equation}
    \mathrm{Pr}(\beta_{n,j}h_n<z) = \mathrm{Pr}(h_n<z)
\end{equation}

Therefore, $\beta_{n,j}h_n \sim \mathcal{CN}(0,\sigma^2)$. We conclude that the columns of the data  matrix $\bY\in\mathbb{C}^{M\times J}$ are independent complex zero mean multivariate Gaussian. As a consequence, the columns of $\Tilde{\bS}$ can be regarded as statistically independent complex Gaussian vector with zero mean.
